# Supplementary material for: Neural architecture impact on identifying temporally extended Reinforcement Learning tasks
Source: arXiv:2310.03161 source file (2023-10-04)
Supplement: Supplementary file 1 [file appendix_a.tex]

\subsection{TimeSformer architecture: Visualization of spatio-temporal attention matrix}
In this section, we visualize the attention probability matrix \texttt{attn\textunderscore sp\textunderscore temp} \in $ \mathbf{R}^{heads \times h.w \times klen.h.w}$ for Joint Space-Time attention model, where $klen$ represents the total sequence length including current token and cached memory tokens, $(h,w)$ the image dimensions. In Section \ref{sec:joint_spt_image_visualization}, we project the attention matrix \texttt{attn\textunderscore sp\textunderscore temp} to respective frames, whereas here we just normalize and convert \texttt{attn\textunderscore sp\textunderscore temp} to heat map. Sum of the probability matrix \texttt{attn\textunderscore sp\textunderscore temp} along each row equals one and there are $(h.w)$ number of such rows, with each row representing one pixel. We normalized the attention matrix in the range $[0,1]$ w.r.t to maximum attention value per head, using Equation \ref{eq:attention_visual_normalization}. \\[0.1in]

Three attention head values are visualized(Figure: [\ref{fig:vit_joint_3d_attention}]) for 30 consecutive time steps, trained with Joint Space-Time model on Pong environment. Time increases from $t$ at top row to $t + 30$ at last row. At the start of a rally, when a ball is introduced in the Pong environment, attention is spread out all over the entire $klen=101$ number of frames as seen from the top-most rows. As the time progresses along the columns, one could observe multiple high attention regions represented by red bands and lower attention regions by scattered yellowish and green segments. Towards the end of the rally, attention clouds are again dispersed around time $\sim (t + 30)$ over the bottom rows (A learned Pong agent playing optimally, took approximately around 30 timesteps to finish a rally).

\begin{figure}[hbt!]
    \centering
    \includegraphics[width=1.0\textwidth]{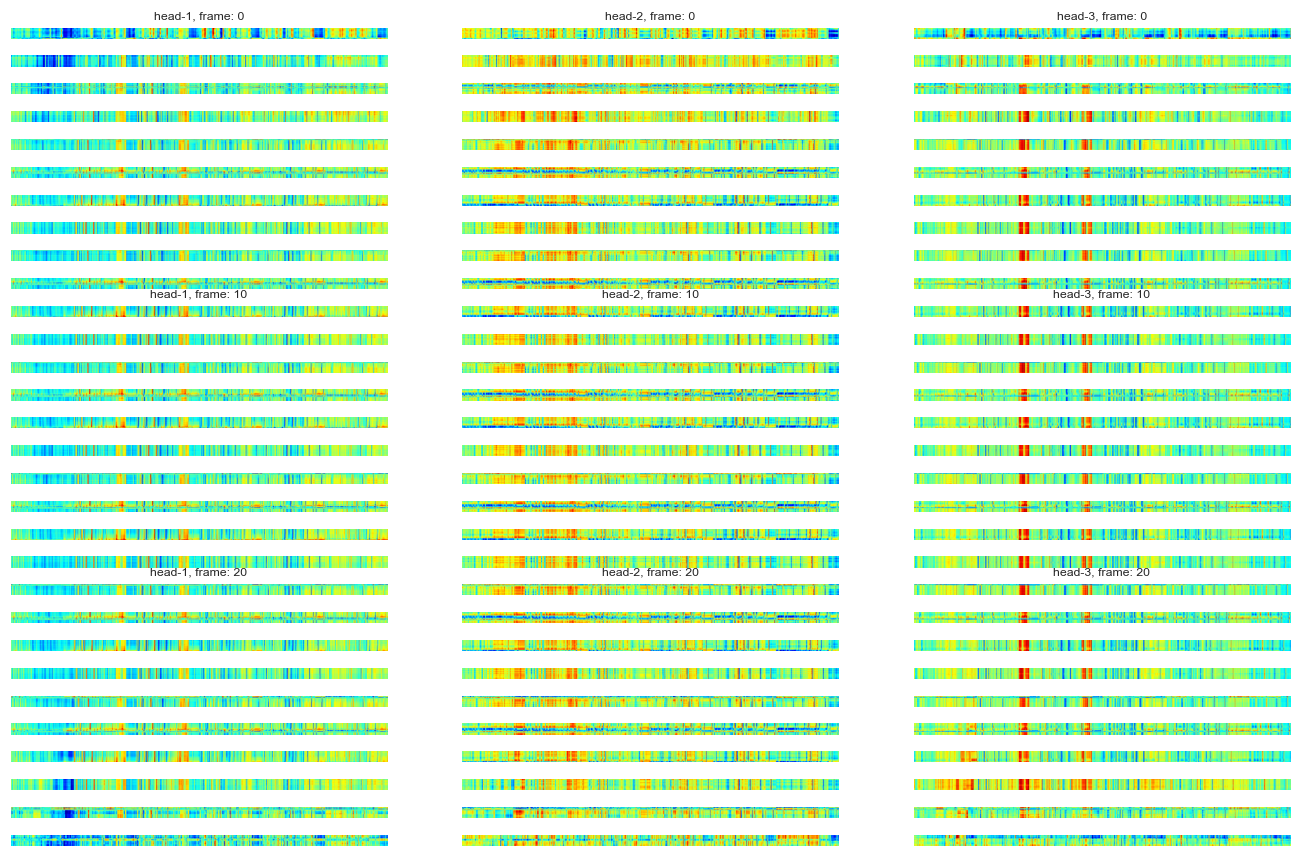}
    \caption{Visualisation of attention heads 1, 2 and 3 for 30 consecutive time steps for Atari Pong environment with Joint Space-Time model (Figure \ref{fig:vit_attention_scheme} Left).}
    \label{fig:vit_joint_3d_attention}
\end{figure}
